# Supplementary material for: Shape Transitions and Chiral Symmetry Breaking in the Energy Landscape of the Mitotic Chromosome
Source: arXiv:1511.03300 source file (2015-11-10)
Supplement: Supplementary file 1 [file suppinfor_BZ_PGW_reduce_size.pdf]

# Supporting Information for "Shape Transitions and Chiral Symmetry Breaking in the Energy Landscape of the Mitotic Chromosome"

Bin Zhang[a,b] and Peter G. Wolynes[a,b,c*]
*Department of [a]Chemistry and [c]Physics and Astronomy, and [b]Center for Theoretical Biological Physics, Rice University, Houston, TX 77005*

## CONTACT PROBABILITY MATRIX FROM HIC DATA

Genome wide chromosome conformation capture (HiC) data for HeLa cell at both G1 (interphase) phase and metaphase from Ref. 1 were downloaded from ArrayExpress database with accession no. E-MTAB-1948. These HiC summary files were then processed to build contact frequency maps using the software package HiCLib (https://bitbucket.org/mirnylab/hiclib) following the protocol outlined in Ref. 2. Data from both replicas were combined together to improve the statistics of detected contacts. A set of filtering protocols were applied to remove very large and small fragments, and to remove the top 0.5% of fragments with the greatest number of reads. Following the construction of the raw matrix, an iterative correction procedure was performed to remove biases that may arise from DNA sequencing or restriction site density.

To determine contact probabilities from the corrected HiC contact frequencies, we normalized the matrix by diagonal elements following the same protocol explained previously [3]. The rationale of this normalization is that neighboring bonded genomic loci are assumed to be in contact with probability one, i.e., $c(i, i+1) \equiv 1$. The resulting raw contact probability matrix is noisy, leading to large fluctuations among neighboring contact probabilities (See Figure S9 (c)). We further smoothed the contact probability matrix with a modified ridge estimator algorithm. As shown in Figure S9, this smoothing has no noticeable effect on the power law scaling of the map, nor does it affect the first 20 dominant eigenvalues and eigenvectors.

## CHROMOSOME MODELS FROM THE MAXIMUM ENTROPY PRINCIPLE

Chromosomes were modeled as beads on a string with the potential energy function

$$U_{\mathrm{ME}}(r) = U(r) + \sum_{ij} \alpha_{ij} f(r_{ij}), \tag{S1}$$

where $U(r)$ is the potential of a homopolymer that includes $U_{\mathrm{FENE}}, U_{\mathrm{angle}}, U_{\mathrm{hc}}, U_{\mathrm{sc}}$ and $U_{\mathrm{c}}$ as defined in Ref. 3. The second term describes contact potentials between pairs of genomic loci, the contact probabilities of which the model aims to reproduce. The contact function is given by $f(r_{ij}) = \frac{1}{2}(1 + \tanh(r_{\mathrm{c}} - r_{ij}))$, with $r_{\mathrm{c}} = 2.0$. $\{\alpha_{ij}\}$ are Lagrangian multipliers that can be determined with an iterative procedure [3]. As shown in Ref. 3 and explained in the main text, this particular form of potential energy function can be derived following the maximum entropy principle, and is the least biased model whose ensemble averages reproduce the experimental pair-wise contact probabilities, i.e., $\langle f(r_{ij})\rangle = f_{ij}^{\mathrm{exp}}$. An intrinsic assumption of the proposed maximum entropy approach is that the set of chromosome structures captured from a population of cells in the HiC experiment can be characterized with an equivalent equilibrium thermodynamic ensemble. Though chromosomes must live in a non-equilibrium environment due to the active processes occurring inside the cell nucleus, as found in many studies [4, 5], effective equilibrium models are often found to provide a good approximation for non-equilibrium systems.

The chromosome consists of 812 beads, each one of which represents 100-kilo base pairs. Resolution of the chromosome model is limited mostly by the statistics of the HiC experiments; below 100 kb, the contacts detected in the experiments exhibit large fluctuations. The total length of the chromosome is therefore of 81.2 Mb. We chose this particular length to model a large segment of chromosome 4 in the q-arm, from 60 Mb to 141.2 Mb, for which the HiC data are of good quality. Particularly, we note that this region does not suffer from the lack of data from the centromere due to the difficulty in sequence alignment. We note that this segment is sufficiently long to investigate complete chromosomes. It is comparable in total length to the full chromosome 17.

## DERIVATION OF THE TAD-AUGMENTED IDEAL CHROMOSOME MODEL

The TAD-augmented ideal chromosome potential defined in Eq. [3] in the main text can be derived following the maximum entropy principle as well. In this case, the external constraints are defined by the average contact probabilities at a given genomic distance $l$

$$\left\langle \sum_i f(r_{i,i+l}) \right\rangle = \sum_i f_{i,i+l}^{\mathrm{exp}}, \quad \text{for } l = 1, \cdots, N, \tag{S2}$$

and the average contact probabilities between genomic loci from two topologically associating domains A and B

$$\left\langle \sum_{i\in A}\sum_{j\in B} f(r_{ij}) \right\rangle = \sum_{i\in A}\sum_{j\in B} f_{ij}^{\exp}, \quad \text{for } A = 1, \cdots, N_t \text{ and } B = A, \cdots, N_t, \tag{S3}$$

where $N$ is the number of genomic loci and $N_t$ is the number of topologically associating domains (TAD). Starting from a homopolymeric model $U(r)$, the chromosome model that satisfies the two sets of constraints shown above while simultaneously maximizing the entropy is the expression shown in Eq. [3] of the main text.

## PARAMETERS IN CHROMOSOME MODELS FROM ITERATIVE OPTIMIZATION

The contact probability map provides a total of $\frac{N\times(N-1)}{2}$ unique pair of contacts. In principle, all these contacts can be included as external constraints in the potential energy function of the chromosome model defined in Eq. S1. For practical reasons, we used the following protocol to select only a fraction of these contacts. First, we only selected pairs from the grid $(1:2:N)\times(1:2:N)$. For example, for locus 1, we only selected contact pairs $(1,3),(1,5),(1,7)$ and so on. This reduces the total number of contacts by a factor of four. Second, we excluded all the pairs that are separated more than 40 Mb apart. Most of these pairs have contact probabilities less than 0.01 and therefore are subject to large experimental noise. It is important to emphasize that all the quantitative comparisons shown in Figure 1 of the main text, and Figures S1-S3 were carried out using the full contact matrices with all pairs being included. The good agreement between simulated and experimental contact matrices shown in these figures suggests that the portion of contact pairs we have selected is sufficient to reproduce the full contact matrix.

For the TAD-augmented ideal chromosome model, we included all pairs with genomic distance less than 40 Mb when calculating the averages defined in Eqs. S2 and S3, and correspondingly, the second and third terms in Eq. [3] of the main text.

The set of parameters $\{\alpha_{ij}\}$ in Eq. [1] and $\{\alpha_{\text{ideal}}\},\{\alpha_{AB}\}$ in Eq. [3] of the main text were determined using the same iterative optimization protocol proposed in Ref. 3. We again used the expression $\xi = \sum_i |\langle f_i\rangle - f_i^{\exp}| / \sum_i f_i^{\exp}$ to measure the convergence of the optimization. Here $i$ refers to the pairs of genomic loci included in Eq. S1 for the direct inversion model; for the augmented ideal chromosome model, $i$ refers to each individual average defined in Eqs. S2 and S3. For the direct inversion, the optimization was stopped when $\xi < 0.2$; for the augmented ideal chromosome model, the optimization was stopped when $\xi < 0.1$.

TABLE I. Simulation parameters of various optimization schemes.

| | | $N_e$ | $N_r$ |
|---|---|---|---|
| Direct Inversion | Interphase | 30 million | 20 |
| | Metaphase | 2 million | 200 |
| TAD-augmented Ideal chromosome | Interphase | 30 million | 10 |
| | Metaphase | 2 million | 50 |

To generate an ensemble of chromosome structures for calculating the average contact probabilities, we used a two-stage simulation protocol that consists of simulated annealing followed by constant temperature equilibration. In the annealing stage, the temperature $T$ was gradually decreased from 8 to 1 over 4 million time steps following a linear schedule. The equilibration stage was initiated from the final structure of the simulated annealing and was carried out with a total of $N_e$ time steps at constant temperature $T = 1$. To further enhance conformational sampling, multiple replicas ($N_r$) starting from different initial structures were independently performed following the two-stage simulation protocol. Table I summarizes the statistics of various optimization schemes.

As seen in Table I, we used more independent replicas for the metaphase chromosome than were used for the interphase to perform the iterative optimization procedure. Our motivation for doing this is that the mitotic chromosome is much more condensed, so that the configurational sampling in each individual replica is limited. Increasing the number of replicas is more effective in expanding the conformational phase space explored by the simulations then is extending trajectory length of each individual replica.

For the TAD-augmented ideal chromosome model, the ideal chromosome potential and the interaction potential among topologically associating domains are not mutually exclusive, since they both contribute to the pair-wise interaction between pairs of genomic loci. The overlap between the two potentials leads to degenerate solutions, and we find that multiple set of $\{\alpha_{\text{ideal}}, \alpha_{AB}\}$ are able to reproduce the experimental contact map equally well. To reduce the degeneracy, we choose the parameter set that maximizes the amplitude of $\alpha_{\text{ideal}}$. To find the largest $\alpha_{\text{ideal}}$ possible that fits the HiC data, we performed three rounds of optimization. Starting from both $\{\alpha_{\text{ideal}}\}$ and $\{\alpha_{AB}\}$ being zero, we determined their values with the first round of iterative optimization. We then scaled the magnitude of $\{\alpha_{AB}\}$ by a factor of 0.1, and performed further optimizations for $\{\alpha_{\text{ideal}}\}$ while keeping $\{\alpha_{AB}\}$ fixed in the second round of optimization. In the final round of optimization, we again allow both $\{\alpha_{\text{ideal}}\}$ and $\{\alpha_{AB}\}$ to vary. We note that the quality of the fit as measured by the agreement between simulated and experimental contact map is not affected by the optimization protocol, consistent with the degeneracy of parameters.

All simulations were performed with Large-scale

Atomic/Molecular Massively Parallel Simulator (LAMMPS). The temperatures of the systems were controlled with Langevin dynamics using a damping coefficient of $10\tau$, where $\tau$ is the reduced time unit. A time step of $0.005\tau$ was used during the annealing step, and $0.01\tau$ was used for the equilibration step.

For the mitotic chromosome, we find that the presence of the confinement potential, $U_c$, has no significant effect on the final chromosome conformations. The reason is that these mitotic structures are smaller than the confinement due to their significant condensation arising from strong contact probabilities. We thus removed this confinement term from the Hamiltonian to improve configurational sampling during the annealing stage of the simulation. Removing the confinement is also consistent with the observation that chromosome territories, which only exist in the interphase and were the motivation for the incorporation of the confinement [6], disappear in the mitotic phase.

## STRUCTURAL CHARACTERIZATION OF CHROMOSOME CONFORMATIONS

### Principal axes

The principal axes of sampled configurations were determined as the eigenvectors of the following covariance matrix

$$\begin{bmatrix} \boldsymbol{xx^T} & \boldsymbol{xy^T} & \boldsymbol{xz^T} \\ \boldsymbol{yx^T} & \boldsymbol{yy^T} & \boldsymbol{yz^T} \\ \boldsymbol{zx^T} & \boldsymbol{zy^T} & \boldsymbol{zz^T} \end{bmatrix} \tag{S4}$$

where $\boldsymbol{x}, \boldsymbol{y}, \boldsymbol{z}$ are row vectors for the position of genomic loci shifted by the mean. For example, $\boldsymbol{x} = (x_1 - \bar{x}, x_2 - \bar{x}, \cdots, x_N - \bar{x})$ with $\bar{x} = \frac{1}{N}\sum_{i=1}^{N} x_i$. The eigenvalues of this matrix correspond to the squared variance $\sigma^2$ of the coordinates along the direction defined by the eigenvectors. Since for a normal distribution, approximately 95% of the points fall in the range of twice the variance, $2\sigma$ provides a good measure for the extension of the structure along each principal axis.

### Twisting variable for chirality

The twisting collective variable $\psi(i)$ is defined with four positions ordered sequentially along the genomic sequence. For a given genomic locus i, we chose the positions based on the four genomic loci, $\{i, i + \frac{1}{2}T, i + \frac{3}{4}T, i + \frac{5}{4}T\}$. Here $T = 25$ Mb corresponds to the period of the most prominent twist observed in the structure. To further smooth out noise, we determined the position of each genomic locus as the center of mass of the nearest in sequence 4 Mb genomic loci, i.e. $(i - 2\text{Mb}) : (i + 2\text{Mb})$, around that locus.

Because the definition of this collective variable requires four genomic loci that span a period of 25 Mb, the twisting variable can only be defined for the genomic loci with index less than $81.2 - \frac{5}{4}T \approx 50$ Mb. This only covers about the first half of the structure. To characterize the second half, we can define the twisting collective variable using the following four genomic loci, $\{i - \frac{5}{4}T, i - \frac{3}{4}T, i - \frac{1}{2}T, i\}$. As shown in Figure S10, the second half exhibits similar behaviors compared to the first half.

### Dihedral angles

Local dihedral angles are defined by four consecutive beads at the resolution of 5 Mb and 10 Mb. For example, at the 5 Mb resolution, the four consecutive beads may be defined as the center of mass of the genomic segments 0-5, 5-10, 10-15 and 15-20 Mb. A biasing potential of the form $\frac{k}{2}(\theta - \theta_o)^2$ was used, with $\theta_o = 90^o$, to enforce torsional preference. We used $k = 0.004\ k_BT$ for the direct inversion and $k = 0.001\ k_BT$ for the augmented ideal chromosome model. Torsional biases were applied to dihedral angles formed by all four consecutive beads at the resolution of both 5 and 10 Mb. These biases were implemented with the software package COLVAR (7).

### Fiber spectrum

To reveal periodically twisting structures at different lengthscales, we calculate the auto-correlation function of displacement vectors $\overrightarrow{v}_i$ along the genomic sequence. The two end points of the vector $\overrightarrow{v}_i$ are defined as genomic loci $i$ and $i + 2$Mb. To smooth out noise, we calculated the position of the end points as the average of a segment of 1 Mb in sequence that are closest to locus $i$ and $i + 2$Mb respectively. Figure S4 shows that the metaphse chromosome structures exhibit long range in sequence correlations when compared with the interphase chromosome. As shown in Ref. 3 and Figure 3(c) of the main text, the Fourier transform of the auto-correlation function is effective in identifying helically twisted structures.

### Topologically associating domains

Topologically associating domains were identified using the breakpoint detection algorithm implemented in the software TADbit [7]. A total of 58 domains were found using the interphase contact map. The boundaries of these domains are provided in the Figure S5 (b), and are plotted on top of the contact map as in Figure S5 (a).

* Correspondence: pwolynes@rice.edu

1. N. Naumova, M. Imakaev, G. Fudenberg, Y. Zhan, B. R. Lajoie, L. A. Mirny, and J. Dekker, Science **342**, 948 (2013).
2. M. Imakaev, G. Fudenberg, R. P. McCord, N. Naumova, A. Goloborodko, B. R. Lajoie, J. Dekker, and L. A. Mirny, Nat Meth **9**, 999 (2012).
3. B. Zhang and P. G. Wolynes, Proc Natl Acad Sci USA **112**, 6062 (2015).
4. S. Wang and P. G. Wolynes, J Chem Phys **135**, 051101 (2011).
5. S. Wang and P. G. Wolynes, J Chem Phys **136**, 145102 (2012).
6. A. Bolzer, G. Kreth, I. Solovei, D. Koehler, K. Saracoglu, C. Fauth, S. Mller, R. Eils, C. Cremer, M. R. Speicher, and T. Cremer, PLoS Biol **3** (2005).
7. D. Bau and M. A. Marti-Renom, Methods **58**, 300 (2012).

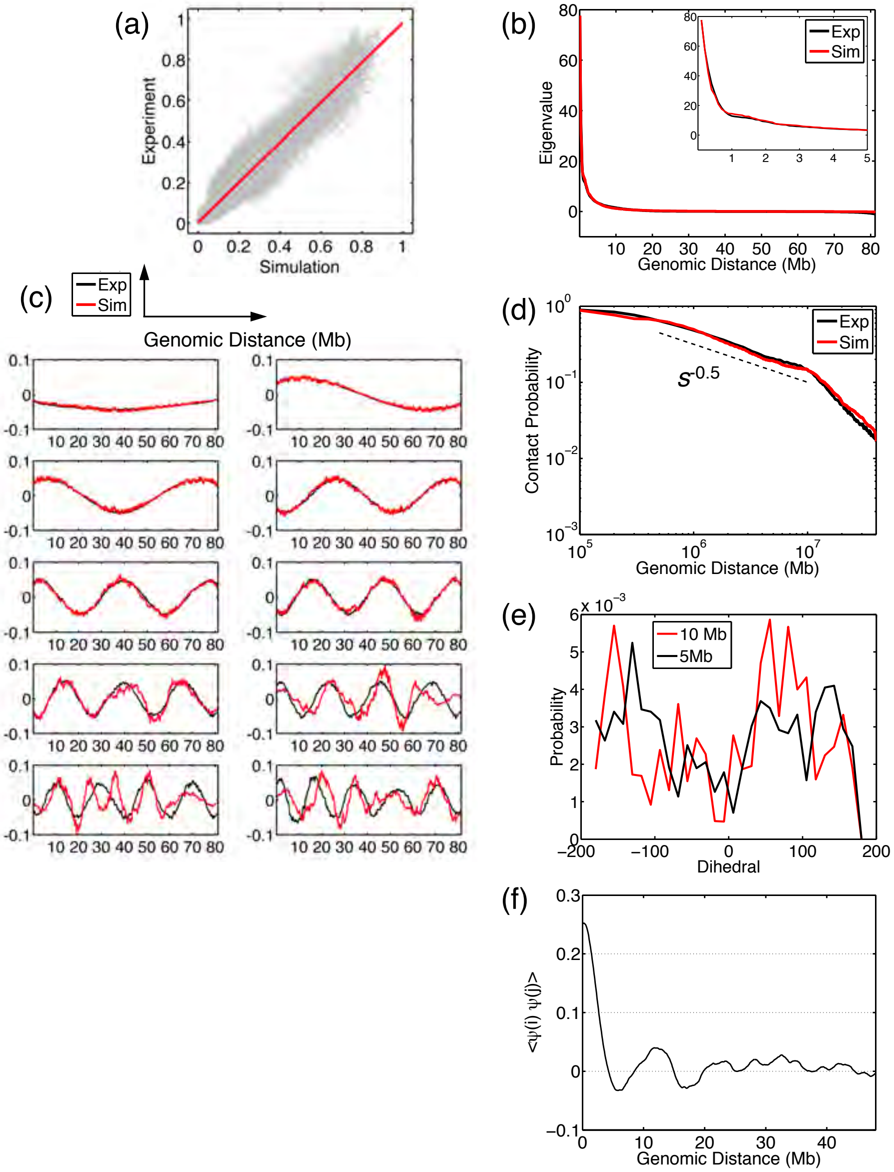


**Figure S1**. Mitotic chromosome model determined from direct inversion. (a) Correlation between the simulated and experimental contact probabilities. The red line is a linear fit to the data, with $a = 0.98$ and $b = 0.00$. R-squared of the fit is 0.93. (b) Comparison of the eigenvalues for the experimental (black) and simulated (red) contact matrices. The inset shows a zoomed-in version of the region with genomic distance less than 5 Mb. (c) Comparison of the top 10 eigenvectors for the experimental (black) and simulated (red) contact matrices. (d) Power law scaling of the experimental (black) and simulated (red) contact probability as a function of genomic distance. (e) Probability distribution of the dihedral angles defined at the resolution of 5 Mb (black) and 10 Mb (red). (f) Autocorrelation of the twist collective variable $\psi(i)$ along the genomic sequence.

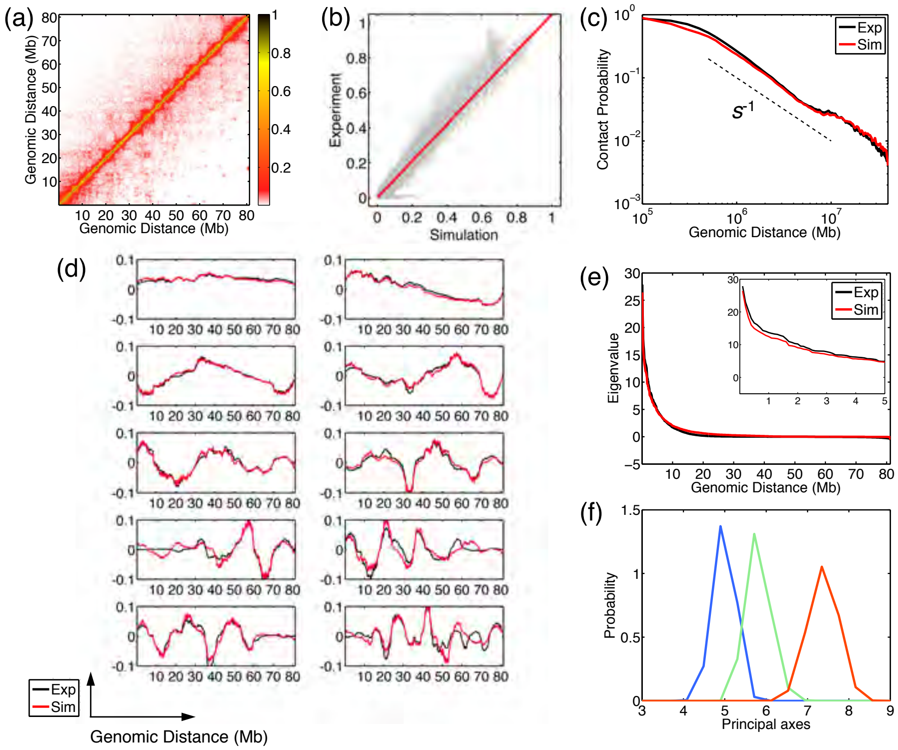


**Figure S2**. Interphase chromosome model determined from direct inversion. (a) Comparison of the experimental (upper triangle) and simulated (lower triangle) contact probability map. (b) Correlation between the simulated and experimental contact probabilities. The red line is a linear fit to the data, with $a = 1.05$ and $b = 0.00$. R-squared of the fit is 0.97. (c) Power law scaling of the experimental (black) and simulated (red) contact probability as a function of genomic distance. (d) Comparison of the top 10 eigenvectors for the experimental (black) and simulated (red) contact matrices. (e) Comparison of the eigenvalues for the experimental (black) and simulated (red) contact matrices. The inset shows a zoomed-in version of the region with genomic distance less than 5 Mb. (f) Probability distribution of extension lengths of interphase chromosome structures along the three principal axes.

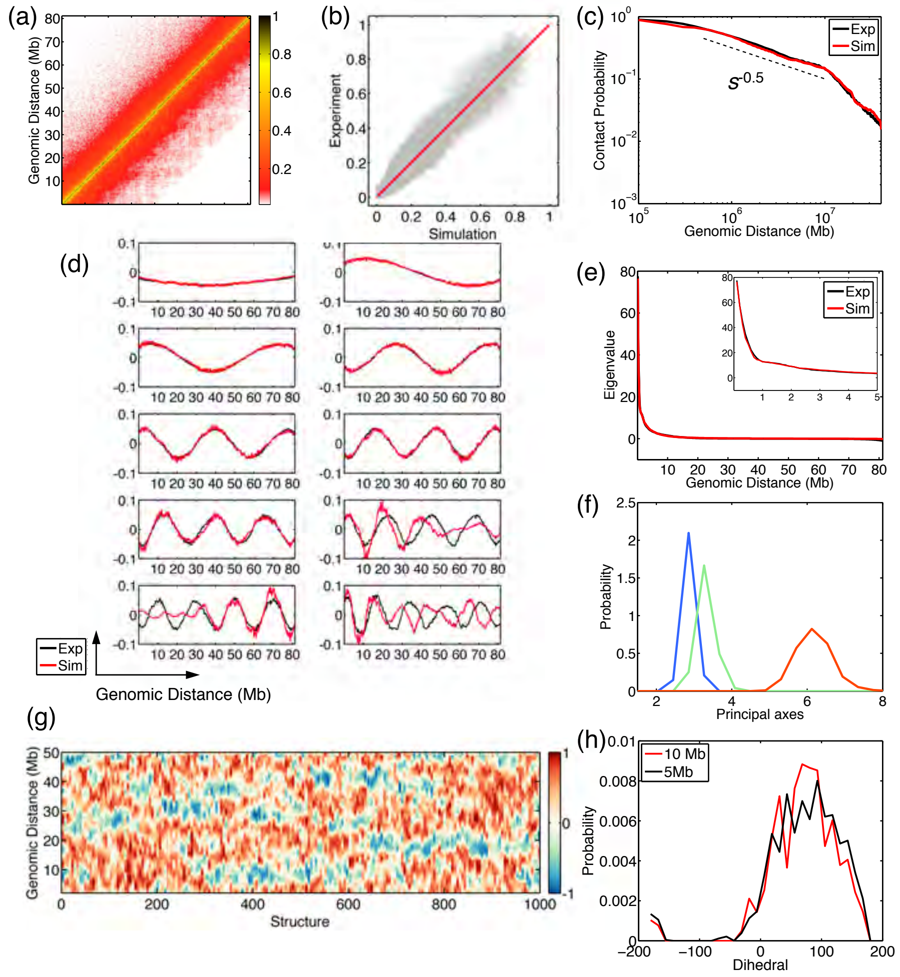


**Figure S3**. Mitotic chromosome model determined from direct inversion with the presence of weak torsional biases. (a) Comparison of the experimental (upper triangle) and simulated (lower triangle) contact probability map. (b) Correlation between the simulated and experimental contact probabilities. The red line is a linear fit to the data, with $a = 0.99$ and $b = 0.00$. R-squared of the fit is 0.95. (c) Power law scaling of the experimental (black) and simulated (red) contact probability as a function of genomic distance. (d) Comparison of the top 10 eigenvectors for the experimental (black) and simulated (red) contact matrices. (e) Comparison of the eigenvalues for the experimental (black) and simulated (red) contact matrices. The inset shows a zoomed-in version of the region with genomic distance less than 5 Mb. (f) Probability distribution of extension lengths of metaphse chromosome structures along the three principal axes. (g) Density plot of the chirality variable $\psi(i)$ along the genomic sequence for different structures from the simulated ensemble. (h) Probability distribution of the dihedral angles defined at the resolution of 5 Mb (black) and 10 Mb (red).

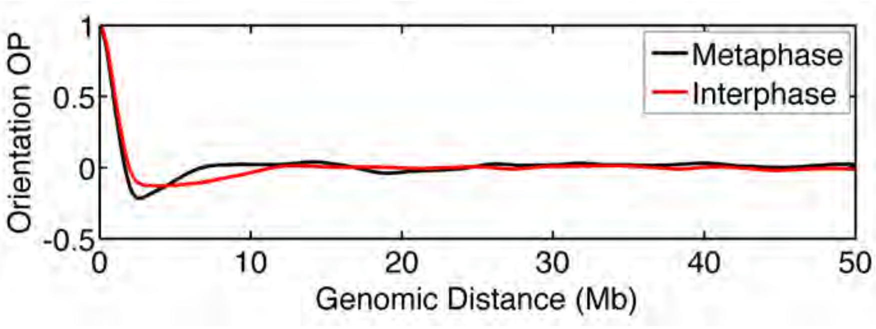


**Figure S4**. Auto-correlation of the orientation vector along the genomic distance for metaphase (black) and interphase (red) chromosome structures.

(a)

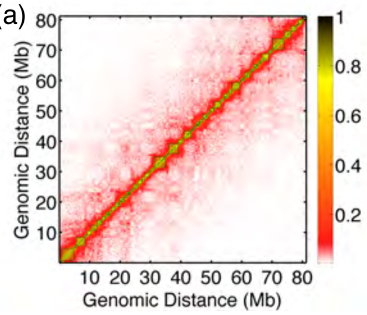


(b)

| Start | End | Start | End | Start | End | Start | End |
|---|---|---|---|---|---|---|---|
| 1 | 6 | 223 | 233 | 410 | 433 | 610 | 627 |
| 7 | 47 | 234 | 238 | 434 | 441 | 628 | 638 |
| 48 | 55 | 239 | 244 | 442 | 449 | 639 | 653 |
| 56 | 84 | 245 | 258 | 450 | 461 | 654 | 663 |
| 85 | 91 | 259 | 272 | 462 | 471 | 664 | 688 |
| 92 | 104 | 273 | 281 | 472 | 488 | 689 | 700 |
| 105 | 123 | 282 | 295 | 489 | 495 | 701 | 738 |
| 124 | 140 | 296 | 300 | 496 | 509 | 739 | 762 |
| 141 | 152 | 301 | 311 | 510 | 531 | 763 | 779 |
| 153 | 166 | 312 | 349 | 532 | 540 | 780 | 784 |
| 167 | 171 | 350 | 354 | 541 | 556 | 785 | 800 |
| 172 | 183 | 355 | 359 | 557 | 568 | 801 | 805 |
| 184 | 198 | 360 | 391 | 569 | 594 | 806 | 812 |
| 199 | 213 | 392 | 404 | 595 | 599 | | |
| 214 | 222 | 405 | 409 | 600 | 609 | | |

**Figure S5**. Topologically associating domains identified using the interphase chromosome contact map. (a) Domains boundaries(green) plotted on top of the interphase chromosome contact map. (b) Boundaries of the identified topologically associating domains with units in 100 kb.

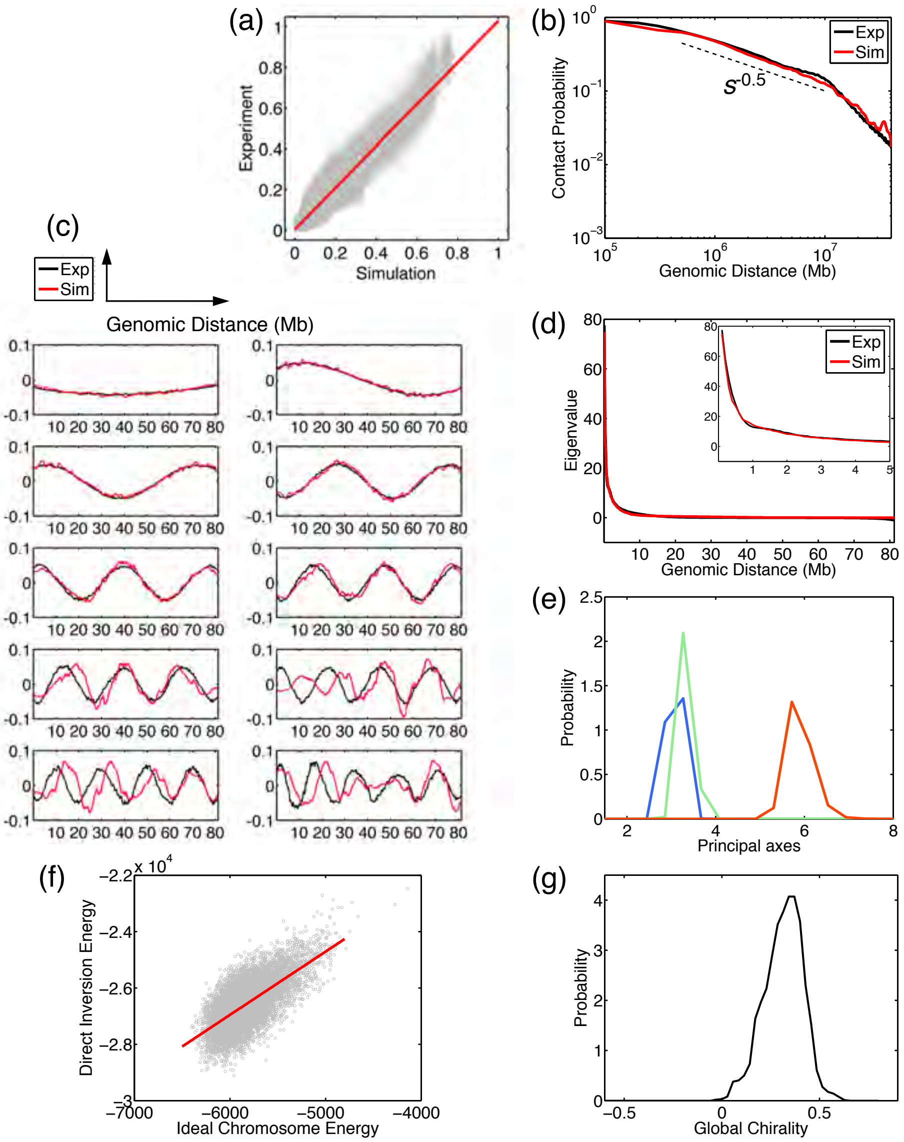


**Figure S6**. Mitotic chromosome model determined from the TAD-augmented ideal chromosome potential with the presence of weak torsional biases. (a) Correlation between the simulated and experimental contact probabilities. The red line is a linear fit to the data, with $a = 1.03$ and $b = 0.00$. R-squared of the fit is 0.93. (b) Power law scaling of the experimental (black) and simulated (red) contact probability as a function of genomic distance. (c) Comparison of the top 10 eigenvectors for the experimental (black) and simulated (red) contact matrices. (d) Comparison of the eigenvalues for the experimental (black) and simulated (red) contact matrices. The inset shows a zoomed-in version of the region with genomic distance less than 5 Mb. (e) Probability distribution of extension lengths of metaphse chromosome structures along the three principal axes. (f) Correlation of the potential energy from the direct inversion with that from the TAD-augmented ideal chromosome model evalulated over an ensemble of chromosome structures simulated using the augmented ideal chromosome model. The red line is a linear fit to the data, and R-squared of the fit is 0.46. (g) Probability distribution of the global chirality for the ensemble of structures.

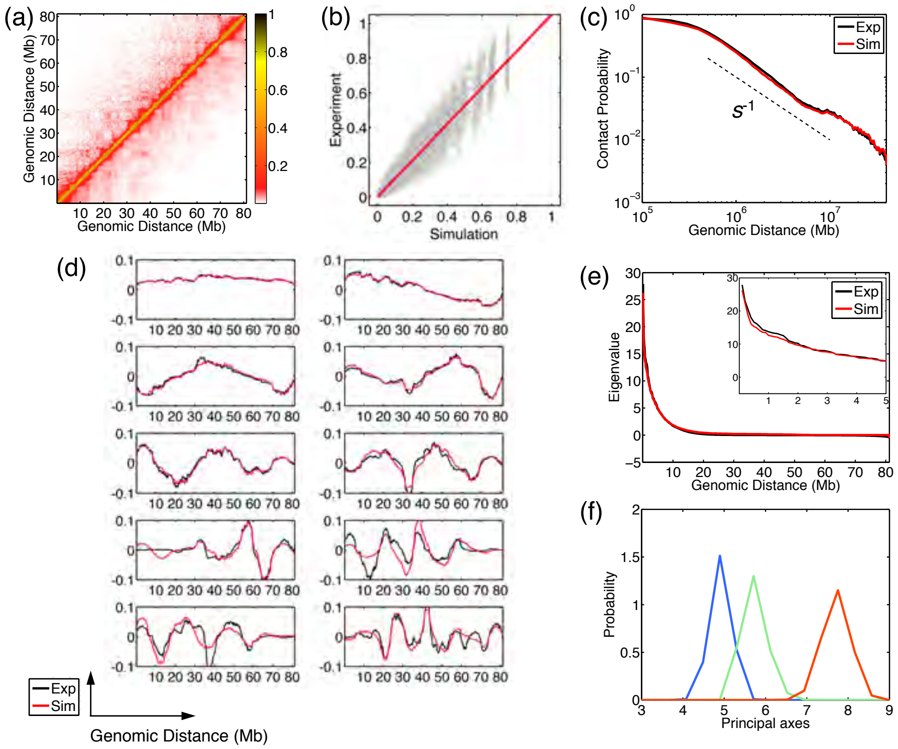


**Figure S7**. Interphase Chromosome model determined from the TAD-augmented ideal chromosome potential. (a) Comparison of the experimental (upper triangle) and simulated (lower triangle) contact probability map. (b) Correlation between the simulated and experimental contact probabilities. The red line is a linear fit to the data, with $a = 0.95$ and $b = 0.00$. R-squared of the fit is 0.94. (c) Power law scaling of the experimental (black) and simulated (red) contact probability as a function of genomic distance. (d) Comparison of the top 10 eigenvectors for the experimental (black) and simulated (red) contact matrices. (e) Comparison of the eigenvalues for the experimental (black) and simulated (red) contact matrices. The inset shows a zoomed-in version of the region with genomic distance less than 5 Mb. (f) Probability distribution of extension lengths of interphase chromosome structures along the three principal axes.

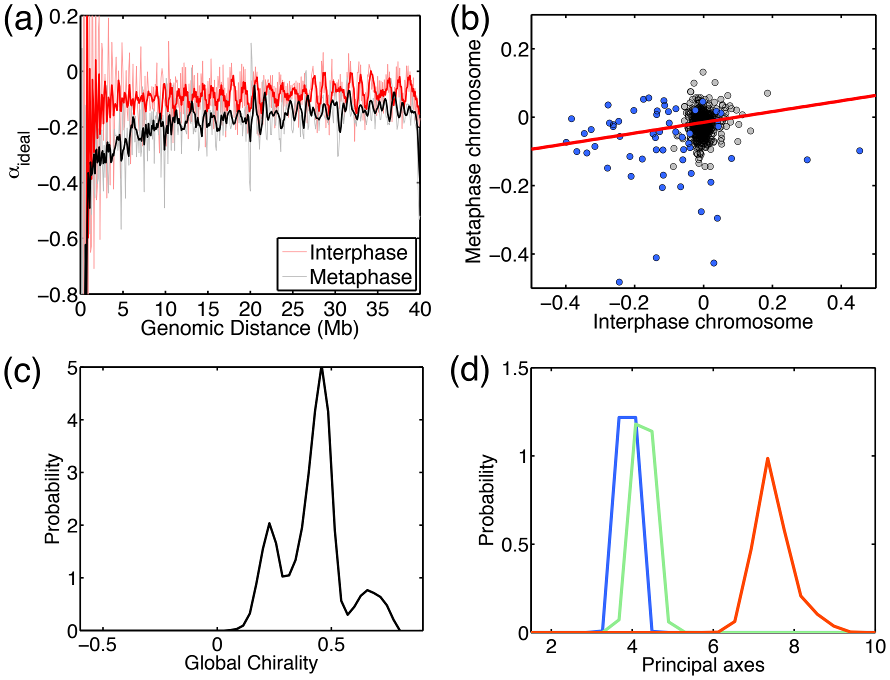


**Figure S8**. Role of the homogenized ideal chromosome potential $\alpha_{\rm ideal}$ in organizing the mitotic chromosome. (a) Comparison between the homogenized ideal chromosome potential for the interphase (red) and metaphase chromosome (black). The darks lines are rolling averages of the raw data (light colors) with a window size of 0.5 Mb. (b) Correlation of the sequence specific interactions among topologically associating domains between the interphase and metaphase chromosomes, with interactions within a domain colored in blue and interactions among domains in grey. The red line is a linear fit to the interphase and metaphse data. (c) Probability distribution of the global chirality for the ensemble of structures simulated using an homogenized ideal potential, i.e., the first two terms in Eq. [3] of the main text, for the mitotic chromosome. (d) Probability distribution of extension lengths along the three principal axes for metaphse chromosome structures simulated using the homogenized ideal chromosome potential.

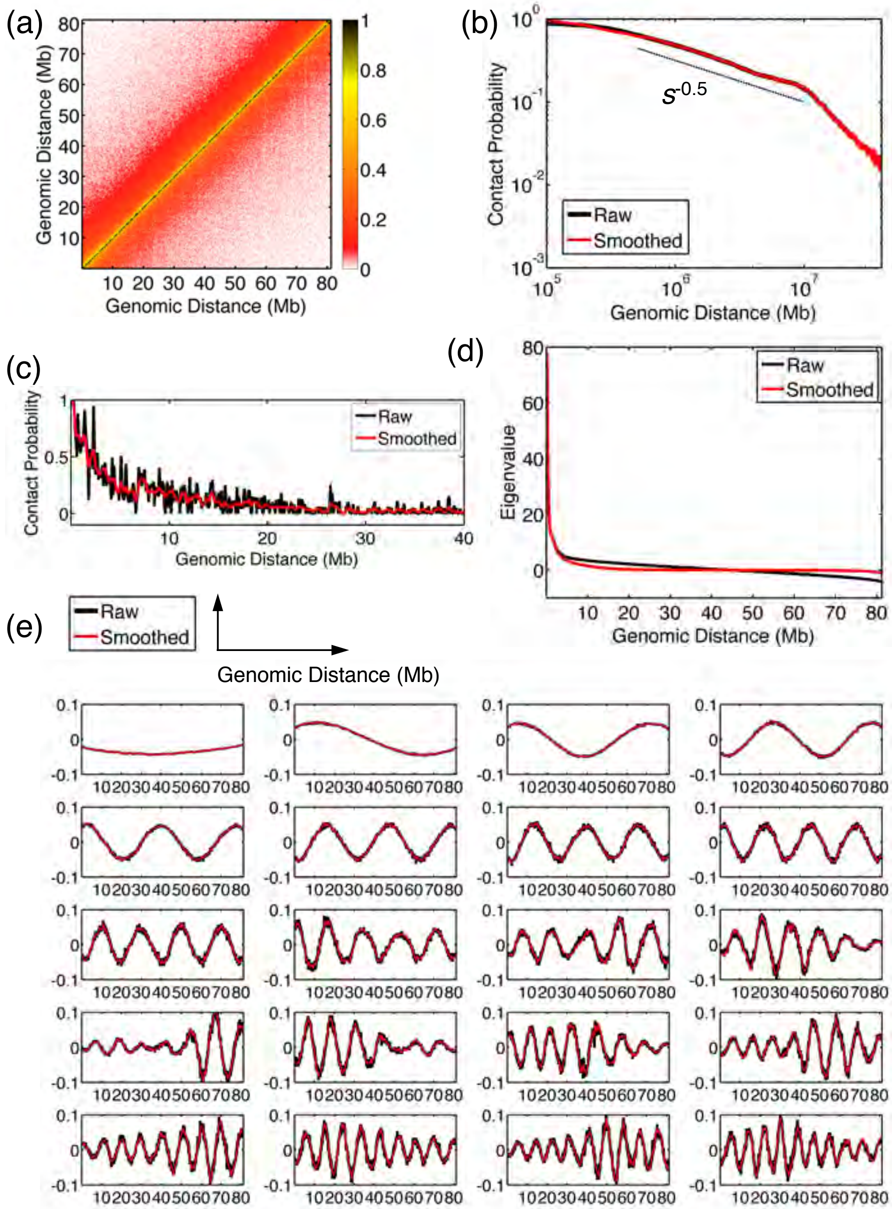


**Figure S9**. Effect of smoothing on the contact probability matrix. (a) Comparison of the smoothed (upper triangle) and raw (lower triangle) contact probability map. (b) Power law scaling of the raw (black) and smoothed (red) contact probability as a function of genomic distance. (c) Detailed comparison of the raw (black) and smoothed (red) contact probabilities. Here we used the probability of locus 1 in contact with other loci as an example. It is clear that there are large fluctuations between neighboring contact probabilities in the raw matrix. (d) Comparison of the eigenvalues for the raw (black) and smoothed (red) contact matrices. (e) Comparison of the top 20 eigenvectors for the raw (black) and smoothed (red) contact matrices.

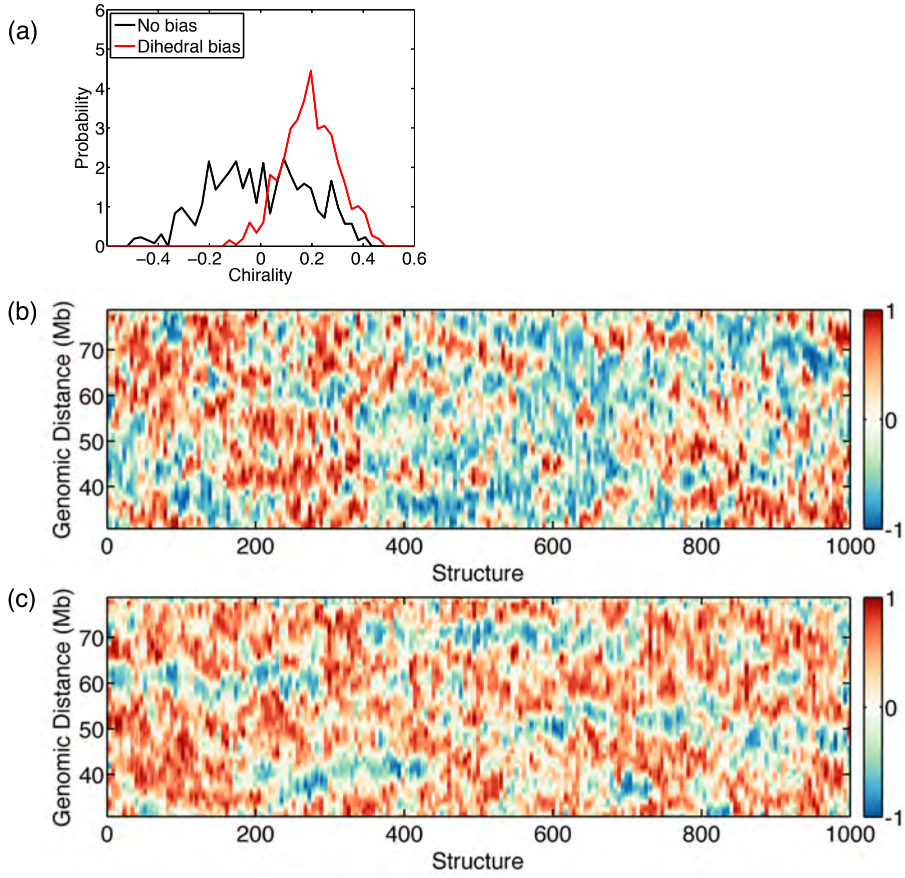


**Figure S10**. Chirality variable measured for the second half of the chromosome. (a) Probability distributions of the global chirality for the ensemble of structures from chromosome models without torsional bias (black) and with torsional bias (red). (b) Density plot of $\psi$ along the genomic sequence for mitotic chromosome structures simulated using the Hamiltonian from direct inversion without torsional bias. (c) Density plot of $\psi$ along the genomic sequence for mitotic chromosome structures simulated using the Hamiltonian from direct inversion with the presence of weak torsional biases.
